# Supplementary material for: MGNet: Monocular Geometric Scene Understanding for Autonomous Driving
Source: arXiv:2206.13199 source file (2022-06-27)
Supplement: Supplementary file 1 [file supplement.pdf]

# MGNet: Monocular Geometric Scene Understanding for Autonomous Driving
# -
# Supplementary Material

Markus Schön Michael Buchholz Klaus Dietmayer
Institute of Measurement, Control and Microtechnology, Ulm University
{markus.schoen,michael.buchholz,klaus.dietmayer}@uni-ulm.de

The supplementary material contains additional visualizations on Cityscapes [2] and KITTI [3], which were not included in the main paper due to space limitations. Furthermore, demo videos of our method on test sequences of both datasets are provided.

## A. Visualizations

Figure 2 shows additional visualizations of our model predictions. In particular, the top block shows examples from the Cityscapes [2] dataset, while the bottom block shows examples from the KITTI [3] dataset. The first four rows in each block show examples where our model performs well. The last row in the top block shows an example with an inaccurate panoptic prediction due to large scale variation in object instances. Thus, the large object is segmented into multiple small instances. Our method shares this weakness with other bottom-up methods, *e.g.* Panoptic DeepLab [1]. The last row in the bottom block shows an example where the depth prediction at the image border is inaccurate. Depth prediction in border regions is very challenging due to camera distortion. Other methods [4, 5] use a post-processing step to combine the depth estimation of the flipped input image with the original one. This improves depth prediction at image borders, but also requires a second forward pass through the model at inference. Since our model focuses on latency, we omit this post-processing step. Additionally, Figure 1 shows top-down views of 3D point cloud predictions corresponding to the top four examples from the KITTI dataset shown in Figure 2.

## B. Demo Videos

We provide demo videos of our method on several test sequences of the Cityscapes and KITTI dataset. The videos show input images overlaid by our respective panoptic prediction and the 3D point cloud with predicted semantic class labels. Predicted instance IDs are omitted in the 3D point cloud for better visualization.

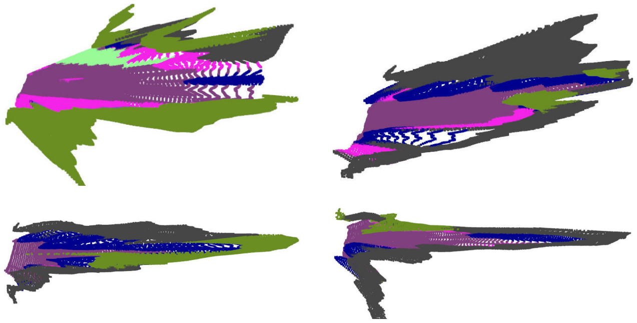

Figure 1: Top-down visualization of 3D point clouds from unseen images from the KITTI [3] dataset.

## References

[1] Bowen Cheng, Maxwell D Collins, Yukun Zhu, Ting Liu, Thomas S Huang, Hartwig Adam, and Liang-Chieh Chen. Panoptic-deeplab: A simple, strong, and fast baseline for bottom-up panoptic segmentation. In *Proceedings of the IEEE/CVF Conference on Computer Vision and Pattern Recognition (CVPR)*, 2020.

[2] Marius Cordts, Mohamed Omran, Sebastian Ramos, Timo Rehfeld, Markus Enzweiler, Rodrigo Benenson, Uwe Franke, Stefan Roth, and Bernt Schiele. The cityscapes dataset for semantic urban scene understanding. In *Proceedings of the IEEE Conference on Computer Vision and Pattern Recognition (CVPR)*, 2016.

[3] Andreas Geiger, Philip Lenz, Christoph Stiller, and Raquel Urtasun. Vision meets robotics: The kitti dataset. *International Journal of Robotics Research (IJRR)*, 2013.

[4] Clement Godard, Oisin Mac Aodha, Michael Firman, and Gabriel J. Brostow. Digging into self-supervised monocular depth estimation. In *Proceedings of the IEEE/CVF International Conference on Computer Vision (ICCV)*, 2019.

[5] Vitor Guizilini, Rares Ambrus, Sudeep Pillai, Allan Raventos, and Adrien Gaidon. 3d packing for self-supervised monocular depth estimation. In *Proceedings of the IEEE/CVF Conference on Computer Vision and Pattern Recognition (CVPR)*, 2020.

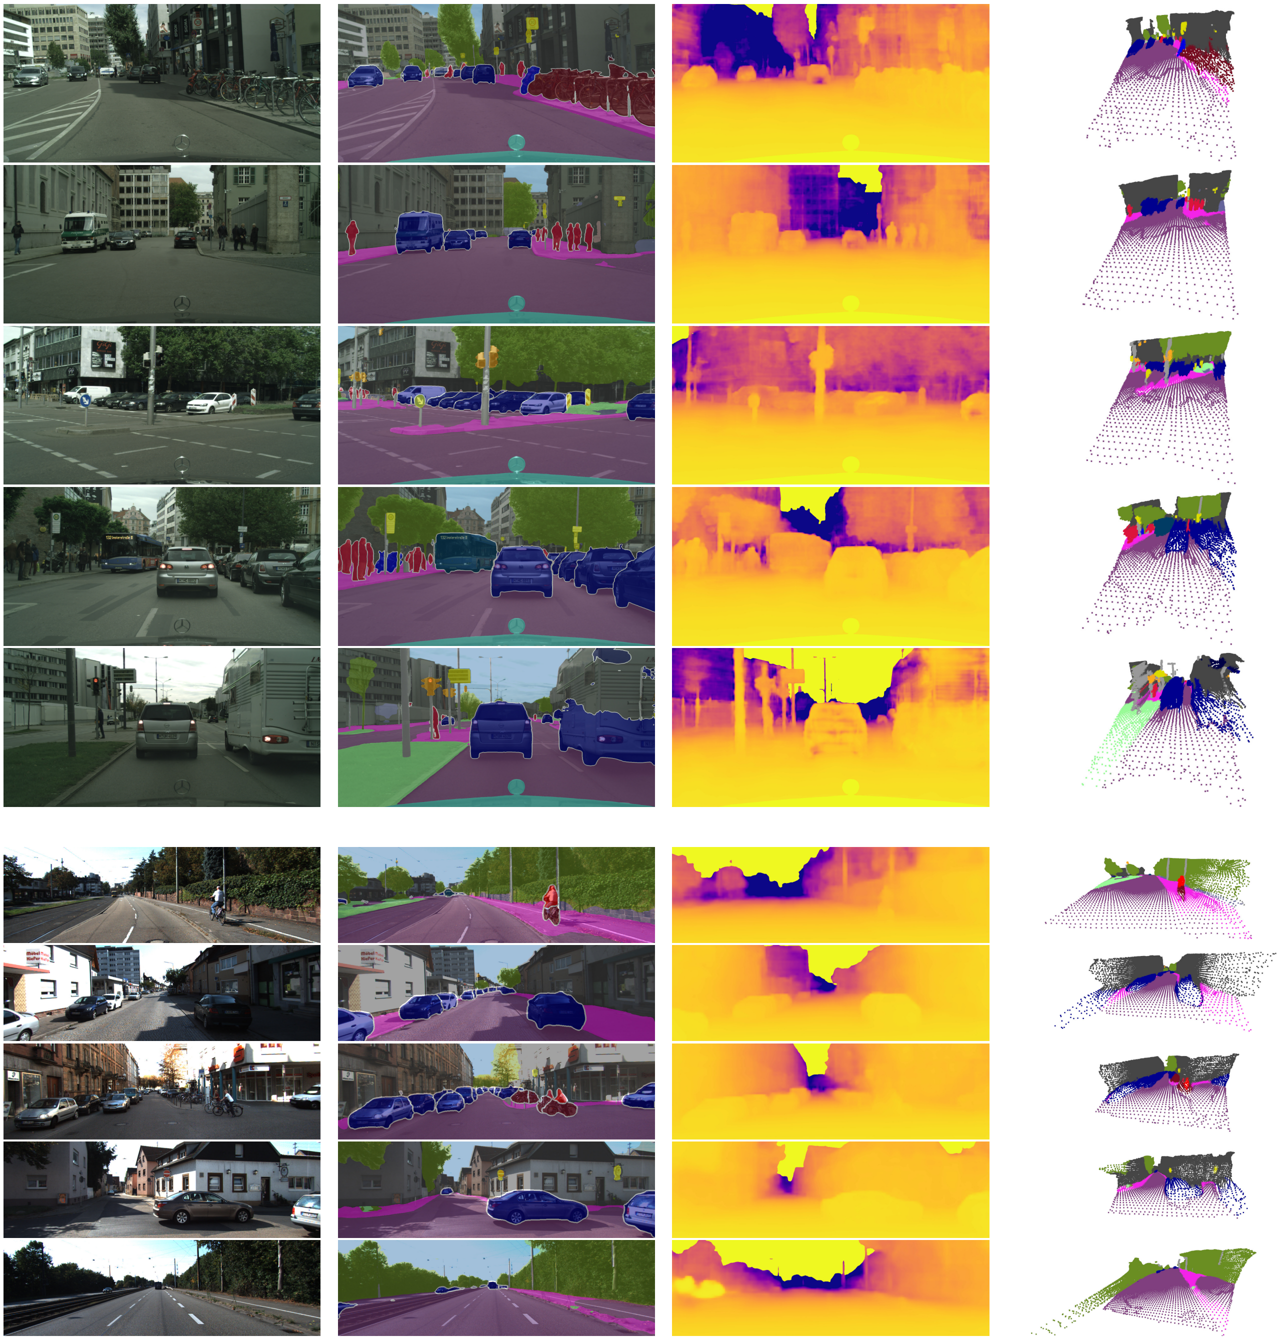

(a) Input image (b) Panoptic segmentation (c) Monocular depth estimation (d) 3D point cloud

Figure 2: More visualizations on unseen images from both datasets. The columns (from left to right) show the input image, the panoptic prediction, the monocular depth estimation, and the final 3D point cloud prediction, respectively. Instances are omitted in the 3D point clouds for better visualization. The top block shows examples from the Cityscapes [2] dataset, while the bottom block shows examples from the KITTI [3] dataset. In both blocks, the last row shows an examples where either the panoptic or depth prediction is not accurate.
